# Supplementary material for: Truth, Lies, and Social Ties: When Image Concerns Fuel Fake News
Source: arXiv:2410.19557 source file (2026-09-15)
Supplement: Supplementary file 1 [file Main_File_Supplementary_Material.tex]

\documentclass[12pt,english]{article}
\usepackage[T1]{fontenc}
\usepackage[latin9]{inputenc}
\usepackage{amsmath}
\usepackage{amsfonts}
\usepackage{natbib}
\usepackage{amsthm}
\usepackage{a4wide}
\usepackage{setspace}
\usepackage{bbm}
\PassOptionsToPackage{hyphens}{url}
\usepackage{hyperref}
\usepackage{geometry}
\usepackage{comment}
\geometry{left=1in,right=1in, top=1in, bottom=1in}
%\makeatletter
%%%%%%%%%%%%%%%%%%%%%%%%%%%%%% Textclass specific LaTeX commands.

\newtheorem{corollary}{Corollary}[section]
\newtheorem{prop}{Proposition}[section]

\newtheorem{lem}{Lemma}[section]
\newtheorem{assume}{Assumption}[section]
\newcommand{\ot}{\tfrac{1}{2}}

\newcommand{\kL}{\kappa(0,L,\tilde{q})}
\newcommand{\mcu}{\mathcal{U}}

%%%%%%%%%%%%%%%%%%%%%%%%%%%%%% User specified LaTeX commands.
\usepackage{pgfplots}

\makeatother

\usepackage{babel}

\linespread{1.5}\selectfont
%\pgfplotsset{compat=1.18}

% Define proposition

\begin{document}

\title{\textbf{Truth, Lies, and Social Ties:\\ When Image Concerns Fuel Fake News}\thanks{Sisak: Erasmus University Rotterdam and Tinbergen Institute. E-Mail: \href{mailto:sisak@ese.eur.nl}{sisak@ese.eur.nl}. Denter: Universidad Carlos III de Madrid. E-Mail: \href{mailto:pdenter@eco.uc3m.es}{pdenter@eco.uc3m.es}. \textcircled{r} indicates randomized order of author names.}}
%Full working paper available here: \url{https://arxiv.org/abs/2410.19557}.}

\author{Dana Sisak \,\textcircled{r}\, Philipp Denter}

\maketitle

\bigskip

\begin{center}
{\Large
\textbf{Online Appendix} 
}
\end{center}

\newpage
\appendix
 
\section{Ability Motive - Additional Results}

\subsection{Equilibrium}

We first show under which conditions a high ability receiver has an incentive to fact check a shared signal. Our next result shows that only surprising/relevant signals will be checked in equilibrium:
\begin{lem}
\label{lem:check}
If $\eta\geq p_R$, a high ability  receiver checks the veracity of a shared signal  if and only if the signal is surprising, $\sigma=0$, and the probability that such a shared surprising signal is fake is strictly positive. If $\eta<p_R$, a high ability receiver never checks a shared signal.
\end{lem}
\begin{proof}
Denote by $\hat{q}$ the belief of a receiver that the shared signal is fake and, slightly abusing notation, by $\hat{p}(\hat{q})$ the updated belief that $\omega=1$ given the shared signal.

\paragraph{$\eta\geq p_R.$}
Assume the receiver received a signal $\sigma=1$. Because $p_R>0.5$, without checking the receiver takes action $a=1$, getting an expected utility of $-(1-\hat{p}(\hat{q}))$. If she checks the signal, with a probability of $\hat{q}$ she learns that the signal is fake and in that case she takes action $a=1$ with belief $\hat{p}(1)=p$. With a probability of $1-\hat{q}$, she learns that the signal is proper, and then she  takes action $a=1$ with belief $\hat{p}(0)$. The difference in expected utilities is
\[
\begin{array}{rcl}
\Delta^1&=&-(1-\hat{p}(\hat{q}))+\hat{q}(1-\hat{p}(1))+(1-\hat{q})(1-\hat{p}(0))\\
&=&-1+\hat{p}(\hat{q})+\hat{q}-\hat{q}\hat{p}(1)+1-\hat{p}(0)-\hat{q}+\hat{q}\hat{p}(0)\\
&=&\hat{p}(\hat{q})-\hat{q}\hat{p}(1)-(1-\hat{q})\hat{p}(0)
\end{array}
\]
Now note that by Bayesian consistency,
\begin{equation}
\label{EQA:BayesianConsitency}
\hat{p}(\hat{q})=\hat{q}\hat{p}(1)+(1-\hat{q})\hat{p}(0)
\end{equation}
But this implies that $\Delta^1=0$. Hence, a high ability sender will never check a signal that is not surprising.

Next assume the receiver received a signal $\sigma=0$. The quality of the signal is lower than $\eta$ because the signal may be fake, and so it is unclear whether the receiver takes action 0 or  1. First assume that without checking the signal is informative enough to induce a belief  $\hat{p}(\hat{q})<\ot$. Then, without checking the signal, she chooses to  takes action $a=0$, yielding an expected utility of $-\hat{p}(\hat{q})$. If she decides to check the signal, she will realize with a probability of $\hat{q}$ that the signal is fake, and hence she would choose to take action $a=1$ with expected utility $-(1-\hat{p}(1))$. If she finds out that the signal is proper, she takes action $a=0$ with an expected utility of $-\hat{p}(0)$. The difference in expected utilities from not checking and checking is
\[
\begin{array}{rcl}
\Delta^0&=&-\hat{p}(\hat{q})+\hat{q}(1-\hat{p}(1))+(1-\hat{q})\hat{p}(0)
\end{array}
\]
Using \eqref{EQA:BayesianConsitency},  this becomes

\[
\begin{array}{rcl}
\Delta^0&=&-\hat{q}\hat{p}(1)-(1-\hat{q})\hat{p}(0)+\hat{q}(1-\hat{p}(1))+(1-\hat{q})\hat{p}(0)\\
&=&-\hat{q}\hat{p}(1)+\hat{q}(1-\hat{p}(1))=\hat{q}(1-2\hat{p}(1))<0
\end{array}
\]
where the last inequality follows from $\hat{p}(1)=p>\ot$. Hence, in this situation it is better to check the signal.

Finally, assume that without checking the signal is not very informative and we have  $\hat{p}(\hat{q})>\ot$. Then, without checking the signal, the receiver chooses to  take action $a=1$, yielding an expected utility of $-(1-\hat{p}(\hat{q}))$. If she decides to check the signal, she will realize that with a probability of $\hat{q}$ the signal is fake, and hence she would  takes action $a=1$ with expected utility $-(1-\hat{p}(1))$. If she finds out that the signal is proper, she takes action $a=0$  with an expected utility of $-\hat{p}(0)$. The difference in expected utilities from not checking and checking is
\[
\begin{array}{rcl}
\Delta^{0'}&=&-(1-\hat{p}(\hat{q}))+\hat{q}(1-\hat{p}(1))+(1-\hat{q})\hat{p}(0)\\
&=&\hat{p}(\hat{q})-1+\hat{q}-\hat{q}\hat{p}(1)+\hat{p}(0)-\hat{p}(0)\hat{q}
\end{array}
\]
Using \eqref{EQA:BayesianConsitency},  this becomes

\[
\begin{array}{rcl}
\Delta^{0'}&=&\hat{q}\hat{p}(1)+(1-\hat{q})\hat{p}(0)-1+\hat{q}-\hat{q}\hat{p}(1)+\hat{p}(0)-\hat{p}(0)\hat{q}\\
&=&(1-\hat{q})\hat{p}(0)-1+\hat{q}+\hat{p}(0)-\hat{p}(0)\hat{q}
\\
&=&2\hat{p}(0)(1-\hat{q})-(1-\hat{q})=(2\hat{p}(0)-1)(1-\hat{q})<0,
\end{array}
\]
where the last inequality follows from $\hat{p}(0)<\ot$. Hence, also in this situation a high ability receiver has an incentive to check the signal.

\paragraph{$\eta< p_R.$}
If $\sigma=1$, we can follow the above steps again to show that a receiver does not have an incentive to check. If $\sigma=0$, as before the quality of the signal is lower than $\eta$ because the signal may be fake. However, because $\eta<p_R$, it is clear now that the receiver takes action 1 independent of the signal's veracity. Without checking the signal,  the receiver chooses to  take action $a=1$, yielding an expected utility of $-(1-\hat{p}(\hat{q}))$.

If she decides to check the signal, she will realize that with a probability of $\hat{q}$ the signal is fake, and hence she would  take action $a=1$ with expected utility $-(1-\hat{p}(1))$. With a probability of $1-\hat{q}$ she finds out that the signal is proper, and she takes also action $a=1$  with an expected utility of $-(1-\hat{p}(0))$. 
The expected utility from checking is 
\[
-\hat{q}(1-\hat{p}(1))-(1-\hat{q})(1-\hat{p}(0))-c_S=-\left(1-\hat{q}\hat{p}(1)-(1-\hat{q})\hat{p}(0)\right)-c_S=-(1-\hat{p}(\hat{q}))-c_S,
\]
where the last steps follows from \eqref{EQA:BayesianConsitency}. This is smaller than $-(1-\hat{p}(\hat{q}))$, and thus the receiver won't check such a signal, either. This proves the lemma.\end{proof}

From Lemma \ref{lem:check} it directly follows that when signals are not sufficiently informative, $\eta<p_R$,  and sharing is costly, $c_S>0$ no sender will share them in equilibrium. Since sharing is costly, a sender only shares a signal if it has the potential to increase status. However, if $\eta<p_R$, then receivers never fact-check any signal, which in turn implies that no sender can gain status from sharing. The next proposition formalizes this intuition:

\begin{prop}
\label{prop:eta_low}
Assume a sender wants to signal her ability to recognize improper signals.
%, as defined in Equation \eqref{EQ:AbilityMotive}. 
If $\eta<p_R$ and $c_S>0$, then there exists a unique not Pareto-dominated equilibrium. In this equilibrium, no information is shared by the sender, and off-equilibrium beliefs satisfy $\pi^{D}\leq \lambda_S+c_S$.
%then there exist off-equilibrium beliefs $\pi^{D}\leq \lambda_S+c_S$ such that no signal is shared in equilibrium. Moreover, any equilibrium with information sharing is Pareto-dominated by this no-sharing equilibrium for $c_S>0$.
\end{prop}

\begin{proof}
We first prove that not sharing is an equilibrium if off-equilibrium beliefs are sufficiently low. Imagine an equilibrium in which no information is shared. Then, along the equilibrium path, both types of senders obtain a status utility of $\lambda_S$. Deviating leads to off-equilibrium social image  belief $\pi^D$ and to deviation utility $\pi^D-c_S$. Hence, there is no incentive to deviate  if and only if  $\lambda_S\geq \pi^D-c_S\Leftrightarrow \pi^D\leq \lambda_S+c_S$. If $\lambda_S+c_S\geq1$, then this is trivially fulfilled for all off-equilibrium beliefs $\pi^D\in[0,1]$. This proves the first part of the proposition.

We next prove that any equilibrium with information sharing is Pareto-dominated by this equilibrium if $c_S>0$. Assume that an equilibrium with information sharing exists. In such an equilibrium, we must have that both types share information with positive probability. If only the high ability type shares, than receivers hold upon observing a shared signal a belief of one, and thus the low ability type would deviate and start sharing. If only the low ability type shares, than receivers hold belief zero. Hence the low type would deviate to not sharing.

Furthermore, both types sharing with positive probability can only be an equilibrium if for both we have $\pi-c_S\geq \pi_\emptyset$, where $\pi$ is the expected social image utility from sharing and $\pi_\emptyset$ the social image utility if no signal is shared. This means that $\pi>\pi_\emptyset$ must hold for any $c_S>0$, which in turn implies that the high ability type needs to share more signals than the low ability type. Thus, the low ability type needs to randomize between sharing and not sharing therefore needs to be indifferent: $\pi-c_S= \pi_\emptyset$. This will also hold for the high ability type. Because a shared signal is more likely to be sent by a high ability type, a not shared signal is more likely to be held by a low type, and therefore $\pi_\emptyset<\lambda_S$. 
But this means that both types' utility is lower in the sharing equilibrium than in the equilibrium without sharing, and hence the sharing equilibrium is Pareto dominated.\end{proof}

\noindent The next Lemma shows which types of equilibria cannot exist for $\eta\geq p_R$:
\begin{lem}
\label{lem:both}
There exists no equilibrium in which one type shares all signals, while the other type chooses not to share some signals, and
%while at the same time one of the types 
one of the types receives expected utility larger than $\lambda_S$.
%, and thus improves their social image. 
%of the two typ[ the low ability sender relays all signals, while the high ability sender keeps some signals. Moreover, except when $\lambda=c$, there exists no equilibrium in which  the high ability sender relays all signals, while the low ability sender keeps some signals.
\end{lem}
\begin{proof}
Assume the low type sender shares all signals, while the high type does not. Then, upon not observing a signal, a receiver's belief about the sender's type being high is 1. But then the low type has an incentive to deviate. This proves the first part of the lemma.

Next assume the high type shares all signals, while the low type does not. This means the high type does not filter signals, and therefore veracity cannot signal status. 
After not observing a signal, status utility is zero, because only the low ability type keeps some signals. 
Note that we need to have $\kL=\kappa(1,L,\tilde{q})<1$. If we had $\kappa(1,L,\tilde{q})\neq \kL$, then the high ability type would share one signal realization  relatively more  frequently than the low ability type, and hence this signal realization would signal status. To see this, assume without loss of generality that $\kappa(1,L,\tilde{q})>\kL$. Then status from sharing $\sigma=0$ is greater than status from sharing $\sigma=1$. But this means the low ability type can gain by deviating to sharing $\sigma=0$ more often. Hence, this cannot be an equilibrium. Therefore, it must be true that $\kappa_{0}=\kappa(1,L,\tilde{q})<1$.

If $\kappa_{0}=\kappa(1,L,\tilde{q})<1$, then sharing any signal realization yields the same status of $\lambda'>\lambda$, and hence a utility of $\lambda'-c_S$. Not sharing yields a status of zero. Therefore, the low ability type has an incentive to deviate to share more signals if $\lambda'>c$. If $\lambda'<c$, then both types have an incentive to deviate and share less.
Only if $\lambda'=c$ could there be an equilibrium in which the high ability sender shares all signals, while the low ability sender keeps some signals to herself. But then both receive an equilibrium utility of zero.
\end{proof}

The intuition for the lemma is as follows. If along the equilibrium path only the high ability type does \textit{not} share some signals, then the low type deviates by keeping all signals for herself. If only the low type keeps some signal for herself, then status after no signal was shared is zero. If sharing costs are low, the low type deviates and shares more signals. If sharing costs are high, the high type deviates and shares no signals. Only if $c_S\geq \lambda_S$ can such an equilibrium exist, but then both types receive zero utility in equilibrium (the low type needs to be indifferent between not sharing and a social image utility of zero, and sharing with sharing costs and positive social image utility). Note that while such a situation is an equilibrium, it is dominated by others. In fact, for both types it is the worst possible outcome. 

\subsection{Welfare}

\subsubsection{Receiver Welfare}
We first study the receivers' welfare in the equilibrium identified in Proposition 1 of the main paper. In particular, we are interested in the effect of sharing costs, which as we have shown in Proposition 2 of the main paper discourage sharing by low ability senders and thus increase the quality of information. Recall that a receiver's utility is zero if her action matches the state and -1 else. Since we assume that fact-checking costs are negligible, our measure of receiver welfare is the probability of a correct choice.

As a first step, we establish a result about how a receiver chooses in equilibrium when the sender decides not to share her signal:

\begin{lem}
\label{lem:choice_no_signal}
If in equilibrium the sender chooses not to share her signal, a  receiver optimally chooses $a=1$. \label{lem:action_nothing_shared}
\end{lem}

\begin{proof}
The probability of not receiving a signal if the state is 1 is
\[
\rho_1^\emptyset=(1-q)\eta+q \left[\beta+(1-\beta)\left(\lambda_S+(1-\lambda_S)\kappa^*(0,L,\tilde{q})\right)\right]
\]
The probability of not receiving a signal if the state is 0 is
\[
\rho_0^\emptyset=(1-q)(1-\eta)+q \left[\beta+(1-\beta)\left(\lambda_S+(1-\lambda_S)\kappa^*(0,L,\tilde{q})\right)\right]<\rho_1^\emptyset.
\]
Hence, upon not receiving a signal, the receiver's posterior increases, implying the posterior must remain above $\ot$. Hence, the chosen action is $a=1$.\end{proof}

The intuition is straightforward. Because a non-surprising signal is never shared, not observing any signal is evidence that the sender's signal was either fake or $\sigma=1$. Because $p_R>\ot$, a receiver's posterior is greater than $\ot$, and therefore the receiver chooses the corresponding action, $a=1$.

Lemma \ref{lem:action_nothing_shared} implies that a high ability receiver chooses action 0  if and only if she receives a proper and surprising signal. Consequently, the probability of a correct choice increases in the amount of surprising signals shared. Since low ability senders share more signals when sharing costs are lower, for the high ability receiver welfare is decreasing in sharing costs. 

Whether a low ability receiver, who cannot distinguish proper from fake surprising signals, chooses action 0 after observing a surprising signal depends on the informativeness of surprising signals. When $\kappa_0^*$ is very small, then mostly high ability senders share surprising signals, meaning they are likely proper. Therefore, if $\kappa_0^*$ is sufficiently small, a low ability receiver chooses $a=0$ when a surprising signal is shared. On the other hand, there are cases where for $\kappa_0^*$ large a low ability receiver chooses $a=1$ also when a surprising signal is shared, as she is too sceptical about the quality of the signal. What does this behavior imply for the welfare of low ability receivers? 

As long as the low ability receiver optimally chooses $a=1$ also when a surprising signal is shared, her welfare is unaffected by sharing costs as her probability of a correct decision stays constant at $p_T$. The interesting case is thus when $\kappa_0^*$ is sufficiently small and a low ability receiver optimally chooses $a=0$ when a surprising signal is shared. The next proposition states our result.

\begin{prop}
\label{prop:WelfareReceiver}
Consider an equilibrium of the form identified in Proposition 1 of the main paper with $\kappa_0^*\in(0,1)$ and assume unbiased receivers $p_R=p_T$. A high ability receiver's welfare strictly decreases in the cost of sharing information $c_S$. A low ability receiver's welfare weakly decreases in the cost of sharing information $c_S$ if 
\[q<\hat{q}\equiv\frac{\eta-p_T}{\beta + \eta+p_T(1 - 2 \beta)  -1 },\]
where $0<\hat{q}<1$, and weakly increases in $c_S$ else.
\end{prop}

\begin{proof}
To prove Proposition \ref{prop:WelfareReceiver}, we study the probability of a correct choice of a low ability receiver who responds to a surprising signal with $a=0$. A low ability receiver who responds to a surprising signal with $a=1$ experiences no change in welfare when $c_S$ changes. The probability of a correct choice of a low ability receiver equals
\[
\begin{array}{rcl}
\Gamma_L&=&p_T \,\mathbb{P}(x=\emptyset|\omega=1)+(1-p_T)\left(1-\mathbb{P}(x=\emptyset|\omega=0)\right),
\end{array}
\]
where 
\[\mathbb{P}(x=\emptyset|\omega=1)=\lambda_S (1-(1-q)(1-\eta)) +(1-\lambda_S)(1-(q(1-\beta)+(1-q)(1-\eta))\kappa^*(0,L,\tilde{q}))\]
denotes the probability of the receiver observing no signal conditional on the state being 1 and 
\[\mathbb{P}(x=\emptyset|\omega=0)=\lambda_S (1-(1-q)\eta) +(1-\lambda_S)(1-(q(1-\beta)+(1-q)\eta)\kappa^*(0,L,\tilde{q}))\]
denotes the probability of the receiver observing no signal conditional on the state being 0.
Taking the derivative with respect to sharing costs $c_S$, we have
 \[
 \begin{array}{rcl}
 \dfrac{\partial \Gamma_L}{\partial c_S}&=&
 p_T\left.\dfrac{\partial  \mathbb{P}(x=\emptyset|\omega=1)}{\partial \kappa(0,L,\tilde{q})}\right|_{\kappa(0,L,\tilde{q})=\kappa^*(0,L,\tilde{q})}\dfrac{\partial \kappa^*(0,L,\tilde{q})}{\partial c_S}\\
 \\
 &-&(1-p_T)\left.\dfrac{\partial \mathbb{P}(x=\emptyset|\omega=0)}{\partial \kappa(0,L,\tilde{q})}\right|_{\kappa(0,L,\tilde{q})=\kappa^*(0,L,\tilde{q})}\dfrac{\partial \kappa^*(0,L,\tilde{q})}{\partial c_S}\\
 \\
 &=&
 -\dfrac{\partial \kappa^*(0,L,\tilde{q})}{\partial c_S}(1-\lambda_S)\left[p_T \left(q(1-\beta)+(1-q)(1-\eta)\right)-(1-p_T)(q(1-\beta)+(1-q)\eta)\right].
 \end{array}
 \]
This derivative is positive if and only if
\[
p_T (q(1-\beta)+(1-q)(1-\eta))>(1-p_T)(q(1-\beta)+(1-q)\eta),
\]
which can be rewritten as $
q>\hat{q}\equiv\frac{\eta-p_T}{\beta + \eta+p_T(1 - 2 \beta)  -1 }$. To show that welfare of low ability receivers may be strictly increasing in $c_S$, we now give a sufficient condition for $a=0$ being the optimal response to a surprising signal. To do this, we show that it is possible that for any $\kappa^*(0,L,\tilde{q})\in[0,1]$ a low ability receiver chooses $a=0$ while $q>\hat{q}$ holds.

The posterior belief of a low type receiver about the state being $\omega=1$ after receiving $\sigma=0$ equals 
\[
\hat{p}_{0\mcu}=\frac{\mathbb{P}(\omega=1|\sigma=0)}{\mathbb{P}(\omega=0|\sigma=0)+\mathbb{P}(\omega=1|\sigma=0)},
\]
where 
\[
\mathbb{P}(\omega=1|\sigma=0)=p_R(\lambda_S (1-q)(1-\eta)+(1-\lambda_S)\left(q (1-\beta)+(1-q)(1-\eta)\right)\kL)
\]
and 
\[
\mathbb{P}(\omega=0|\sigma=0)=(1-p_R)(\lambda_S (1-q)\eta+(1-\lambda_S)\left(q (1-\beta)+(1-q)\eta\right)\kL).
\]
Next note that when $q=0$, then
\[
\left.\hat{p}_{0\mcu}\right|_{q=0}=\frac{p_R(1-\eta)}{p_R(1-\eta)+(1-p_R)\eta}<\ot, 
\]
and when $q=1$, $\left.\hat{p}_{0\mcu}\right|_{q=1}=p_R>\ot$, independent of $\kL$. 
Moreover, $\hat{p}_{0\mcu}$ strictly increases in  $\kL$. Thus, if for $\kL=1$ we have that $\hat{p}_{0\mcu}|_{\kL=1}\leq \ot$, then a low ability receiver always optimally chooses $a=0$. Therefore, we set $\kL=1$ in what follows.
Moreover,  because $\hat{p}_{0\mcu}$ strictly increases  in $q$, 
there must be $\tilde{q}\in(0,1)$ such that $\hat{p}_{0\mcu}\leq \ot\Leftrightarrow q\leq \tilde{q}$.
Solving we find that 
\[
\tilde{q}=\frac{\eta -p_R}{\beta +\eta -(1-\beta) {\lambda_S} (2 {p_R}-1)-2 \beta  {p_R}+{p_R}-1
  )}.
\]
We can conclude that if $q<\tilde{q}$, then $\hat{p}_{0\mcu}<\ot$, and therefore a low ability receiver chooses $a=1$ for any $\kL$. Note that for $p_R=p_T>\ot$, $\hat{q}<\tilde{q}$ which proves that low ability receiver welfare may strictly increase with sharing costs.\end{proof}

We find that the preferences of both types of receivers about sharing costs might diverge. In particular, a low ability receiver may benefit from higher sharing costs as it increases the quality of information shared, while a high ability type strictly prefers lower costs of sharing. In a final step, we study how welfare compares to a situation where a sender never shares her signal (prohibitively high costs of sharing). A high ability type is always better off with information sharing, because she will only base a decision on proper news. But could a low ability receiver suffer due to information sharing? If her belief is correct, $p_R=p_T$, then this is not possible and the probability of her taking a correct decision is weakly greater than with no sharing. She will simply ignore information when the quality of the signal is not high enough. If, however, $p_R\neq p_T$, then information sharing can be both beneficial and detrimental, depending on the parameters of the game.\footnote{This can be illustrated in a simple example. Assume that $p_R<p_T$ and thus receivers are too optimistic about the surprising state of the world. Then a low ability receiver will trust a surprising signal of relatively low quality too quickly and choose $a=0$, even though she should rationally ignore it and choose $a=1$. } This insight is formalized in our next corollary:

\begin{corollary}
\label{cor:highbenefits_lowmaynot}
Consider an equilibrium of the form identified in Proposition 1 of the main paper with $\kappa_0^*\in(0,1)$. A high ability receiver's welfare is strictly higher than in a situation with no information sharing. If $p_R=p_T$, a low ability receiver's welfare is weakly higher than in a situation with no information sharing. However, if $p_R\neq p_T$, then a low ability receiver may be better off with no information sharing.
\end{corollary}

\subsubsection{Sender Welfare}
We formalize the intuitions discussed in the main paper in our next proposition:

\begin{prop}
\label{prop:welf_sender}
The equilibrium utility of a low ability sender (i) strictly decreases in $c_S$ and is (ii) generally strictly lower than $\lambda_S$. When the cost of sharing is low, a high ability sender benefits from information sharing. However, when $c_S$ increases, this may change, and a high ability sender's utility might drop below $\lambda_S$. This is particularly likely when the share of high ability receivers is low and if  surprising news are  likely to be fake.
\end{prop}

\begin{proof}
Consider first a low ability sender. Her expected utility from sharing a surprising signal must be equal to the expected utility from not sharing in equilibrium, where the latter equals
\[
\pi_\emptyset=\frac{\lambda_S(1-z_{0\mathcal{P}}^R)}{\lambda_S(1-z_{0\mathcal{P}}^R)+(1-\lambda_S)\left[(1-z_0^R+z_0^R(1-\kL)\right]}.
\]
This is strictly increasing in $\kL$, which in turn strictly decreases in $c_S$ as long as $\kL>0$. Therefore, the welfare of the low ability sender strictly decreases in $c_S$ as long as she remains active ($\kL>0$). Her welfare is thus greatest when $c_S=0$.  

For the low ability sender's welfare to be larger than $\lambda_s$, it would need to be true that

\[
\begin{array}{c}
\pi_\emptyset>\lambda_S
\Leftrightarrow \dfrac{\lambda_S(1-z_{0\mathcal{P}}^R)}{\lambda_S(1-z_{0\mathcal{P}}^R)+(1-\lambda_S)\left[(1-z_0^R+z_0^R(1-\kL)\right]}>\lambda_S\\
\\
\Leftrightarrow \kL>\frac{z^R_{0\mathcal{P}}}{z_0^R}
\end{array}
\]

If this is true, then 
\begin{equation}
\label{EQ:Delta}
\Delta\equiv u_{0\mathcal{U}}-u_\emptyset
\end{equation}
\noindent is negative. In any equilibrium, in which the low ability sender is active, it needs to be equal to zero. Because $\Delta$ strictly decreases in $\kL$, it follows that the equilibrium value  $\kappa^*$ must be smaller than $\frac{z^R_{0\mathcal{P}}}{z_0^R}$. Therefore, the low ability sender's expected utility must be strictly smaller than $\lambda_S$.

Next consider the high ability sender, and start by focusing on the case of costless information sharing,  $c_S=0$. We just showed that in this case $u_{0\mathcal{U}}=\pi_{\emptyset}<\lambda_S$.
Then it follows from Bayes consistency of the beliefs---the expected posterior must equal the prior---that $u_{0\mathcal{P}}>\lambda_S$. Furthermore, as the expected utility of a low ability sender is strictly less than $\lambda_S$, and thus again by Bayes consistency, the expected utility of a high ability sender needs to be larger than $\lambda_S$. Thus, the high ability sender is better off than without information sharing for $c_S=0$.

From \eqref{EQ:Delta}, by setting $\kL=0$, we can find the critical level of the cost of sharing such that the low ability sender stops sharing altogether. The solution is
\[
\bar{c}_S=\frac{1-{\lambda_R}-{\lambda_S}+{\lambda_R} {\lambda_S} z_{0P}^R}{1-{\lambda_S}
   {z_{0P}^R}}+\frac{{\lambda_R} {z_{0P}^S}}{{z_{0}^S}}
\]
%f surprising news are sufficiently likely to be fake
Note that when $\kL=0$, then the utility of a high ability receiver from sharing a proper surprising signal is
\[
\left.u_{0\mathcal{P}}\right|_{\kL=0}=1-c_S.
\]
Hence, when $c_S=\bar{c}_S$, we have
\[
\left.u_{0\mathcal{P}}\right|_{\kL=0\wedge c_S=\bar{c}_S}=\lambda_R\left(1-\dfrac{{z^S_{0P}}}{{z^S_0}}\right)+\dfrac{\lambda_S
   (1-z^R_{0P})}{1-\lambda_S z^R_{0P}}.
\]
This strictly increases in $\lambda_R$ and it strictly decreases in $z_{0\mathcal{P}}$. To prove the result let $\lambda_R\rightarrow0$, i.e., there are close to zero high ability receivers. In this case,  we get
\[
\left.u_{0\mathcal{P}}\right|_{\kL=0\wedge c_S=\bar{c}_S\wedge \lambda_R=0}=\dfrac{\lambda_S
   (1-z^R_{0P})}{1-\lambda_S z^R_{0P}}.
\]
That is, the status utility of a high ability sender who shares a surprising and proper signal is smaller than $\lambda_S$.
 But note that the utility from not sharing in this case is still strictly below $\lambda_S$, and therefore the ex ante expected utility of a high ability sender must be smaller than $\lambda_S$ as well. This completes the proof.\end{proof}

\section{Worldview -- Additional Results}

\subsection{The Uniform Distribution Satisfies Assumption 1}
We first show that if $F_S$ is uniform on $[\underline{z},\overline{z}]$, then the assumptions made in Proposition 5 are satisfied. Further below, we establish a condition that guarantees uniqueness in symmetric situations.

Under the distributional assumptions, 
\[
\begin{array}{rcl}
\widehat{p}_S^U(0)&=&\frac{p_{Sl}+\underline{z}}{2}\\
\widehat{p}_S^U(1)&=&\frac{p_{Sh}+\overline{z}}{2}\\
\widehat{p}_S^U(\emptyset)&=&\frac{\widehat{p}_R(p_{Sh}^2-\underline{z}^2) +(1-\widehat{p}_R)(\overline{z}^2-p_{Sl}^2)}{2 (\widehat{p}_R(p_{Sh}-\underline{z}) +(1-\widehat{p}_R)(\overline{z}-p_{Sl}))}
\end{array}
\]
In a responsive equilibrium, the following conditions must be equal to zero (see Lemma 1):
%$p_{Sh}>\widehat{p}_S^U(\emptyset)>p_{Sl}$. Otherwise, either $\widehat{p}_S^U(0)=\widehat{p}_S^U(\emptyset)$, or $\widehat{p}_S^U(1)=\widehat{p}_S^U(\emptyset)$, or both. But in a responsive equilibrium, this is not possible, because sharing different signals would not lead to different beliefs. 
%Therefore, the equilibrium conditions become
\[
\begin{array}{rcl}
C_L&=&\frac{p_{Sl}+\underline{z}}{2}-2{p_{Sl}}-c_S+\frac{\widehat{p}_R(p_{Sh}^2-\underline{z}^2) +(1-\widehat{p}_R)(\overline{z}^2-p_{Sl}^2)}{2 (\widehat{p}_R(p_{Sh}-\underline{z}) +(1-\widehat{p}_R)(\overline{z}-p_{Sl}))}\\
C_H&=&2p_{Sh}-\frac{p_{Sh}+\overline{z}}{2}-c_S-\frac{\widehat{p}_R(p_{Sh}^2-\underline{z}^2) +(1-\widehat{p}_R)(\overline{z}^2-p_{Sl}^2)}{2 (\widehat{p}_R(p_{Sh}-\underline{z}) +(1-\widehat{p}_R)(\overline{z}-p_{Sl}))}
\end{array}
\]

We have
%Next we determine comparative statics. We need the following derivatives:
\[
\begin{array}{rcl}
\frac{\partial C_L}{\partial p_{Sl}}&=&\frac{(1-\widehat{p}_R) \left(\widehat{p}_R \left(p_{Sh}^2-2 p_{Sh}
   p_{Sl}-(p_{Sl}-{\overline{z}})^2+2 p_{Sl}
   {\underline{z}}-{\underline{z}}^2\right)+(p_{Sl}-{\overline{z}})^2\right)}{2
  (\widehat{p}_R(p_{Sh}-\underline{z}) +(1-\widehat{p}_R)(\overline{z}-p_{Sl}))^2}-\frac{3}{2}<0\\
\frac{\partial C_H}{\partial p_{Sh}}&=&\frac{3}{2}-\frac{\widehat{p}_R \left(\widehat{p}_R \left(p_{Sh}^2+2
   p_{Sh}
   (p_{Sl}-{\overline{z}}-{\underline{z}})-p_{Sl}^2+{\overline{z}}^2+{\underline{z}}^2
   \right)-2 p_{Sh} p_{Sl}+2 p_{Sh}
   {\overline{z}}+p_{Sl}^2-{\overline{z}}^2\right)}{2 (\widehat{p}_R(p_{Sh}-\underline{z}) +(1-\widehat{p}_R)(\overline{z}-p_{Sl}))^2}>0\\
\end{array}
\]
The inequalities follow from the derivatives being monotone in $\widehat{p}_R$, and then it is easy to show that $\frac{\partial C_L}{\partial p_{Sl}}\in[-\frac{3}{2},-1]$ and $\frac{\partial C_H}{\partial p_{Sh}}\in[1,\frac{3}{2}]$.

If we can show that also  $\text{det}\, M<0$, where
\[
  M=
  \left(
  \begin{array}{cc}
  \frac{\partial C_L}{\partial p_{Sl}}&\frac{\partial C_L}{\partial p_{Sh}}\\
  \frac{\partial C_H}{\partial p_{Sl}}&\frac{\partial C_H}{\partial p_{Sh}}
  \end{array}\right)   
\]
then we have shown that under the assumption of uniform sender types the assumptions used in the proof  of Proposition 5 are satisfied.
\begin{comment}

as well as
\[
\begin{array}{cc}
 M_L^1=
  \left(
  \begin{array}{cc}
  -\frac{\partial C_L}{\partial \widehat{p}_R}&\frac{\partial C_L}{\partial p_{Sh}}\\
  -\frac{\partial C_H}{\partial \widehat{p}_R}&\frac{\partial C_H}{\partial p_{Sh}}
  \end{array}\right)  &
  M_H^1=
  \left(
  \begin{array}{cc}
  \frac{\partial C_L}{\partial p_{Sl}}&-\frac{\partial C_L}{\partial \widehat{p}_R}\\
  \frac{\partial C_H}{\partial p_{Sl}}&-\frac{\partial C_H}{\partial \widehat{p}_R}
  \end{array}\right)  \\
  &\\
 M_L^c=
  \left(
  \begin{array}{cc}
  -\frac{\partial C_L}{\partial c_S}&\frac{\partial C_L}{\partial p_{Sh}}\\
  -\frac{\partial C_H}{\partial c_S}&\frac{\partial C_H}{\partial p_{Sh}}
  \end{array}\right)  &
  M_H^c=
  \left(
  \begin{array}{cc}
  \frac{\partial C_L}{\partial p_{Sl}}&-\frac{\partial C_L}{\partial c_S}\\
  \frac{\partial C_H}{\partial p_{Sl}}&-\frac{\partial C_H}{\partial c_S}
  \end{array}\right)  
\end{array}
\]
Then $\frac{\partial p_{Sl}}{\partial \widehat{p}_R}=\frac{\left|M_L^1\right|}{\left|M\right|}$, $\frac{\partial p_{Sh}}{\partial \widehat{p}_R}=\frac{\left|M_H^1\right|}{\left|M\right|}$, $\frac{\partial p_{Sl}}{\partial c_s}=\frac{\left|M_L^c\right|}{\left|M\right|}$, and $\frac{\partial p_{Sh}}{\partial c_S}=\frac{\left|M_H^c\right|}{\left|M\right|}$.
\end{comment}
We can calculate $|M|$ directly:
\[
|M|=-\frac{3 \left(K_1 p_R+K_2 p_R^2+2
   (p_{Sl}-\overline{z})^2\right)}{4 (p_R
   (p_{Sh}+p_{Sl}-\overline{z}-\underline{z})-p_{Sl}+\overline{z})^2}
\]
where
\[
K_1=-p_{Sh}^2-2 p_{Sh} p_{Sl}+4 p_{Sh} \overline{z}-5
   p_{Sl}^2+8 p_{Sl} \overline{z}+4 p_{Sl} \underline{z}-3
   \overline{z}^2-6 \overline{z} \underline{z}+\underline{z}^2
\]
and
\[
K_2=3 p_{Sh}^2+2 p_{Sh} (p_{Sl}-2 (\overline{z}+\underline{z}))+3
   p_{Sl}^2-4 p_{Sl} (\overline{z}+\underline{z})+\overline{z}^2+6
   \overline{z} \underline{z}+\underline{z}^2
\]
We aim to show that $|M|<0$. Because $K_2<0$ and $\widehat{p}_R\in[0,1]$, if
\[
-\frac{3 \left({K_1} \widehat{p}_R+{K_2} \widehat{p}_R+2
   (p_{Sl}-\overline{z})^2\right)}{4 (\widehat{p}_R
   (p_{Sh}+p_{Sl}-\overline{z}-\underline{z})-p_{Sl}+\overline{z})^2}=-\frac{3 \left(p_R (p_{Sh}+p_{Sl}-\overline{z}-\underline{z})
   (p_{Sh}-p_{Sl}+\overline{z}-\underline{z})+(p_{Sl}-\overline{z})^2\right)}{2 (p_R
   (p_{Sh}+p_{Sl}-\overline{z}-\underline{z})-p_{Sl}+\overline{z})^2}<0
\]
then also $|M|<0$. This inequality holds iff $
p_R (p_{Sh}+p_{Sl}-\overline{z}-\underline{z})
   (p_{Sh}-p_{Sl}+\overline{z}-\underline{z})+(p_{Sl}-\overline{z})^2>0$.
Now note that this is least likely to hold if $p_R=1$, in which case the inequality simplifies to $(p_{Sh}-\underline{z})^2>0$. Hence, indeed $|M|<0$, and therefore the assumptions we used in the proof of Proposition 5 are satisfied when sender types are uniform.

\bigskip
\subsection{Bounds on the Elasticity of $F_S$ in Symmetric Games}
Next we show how uniqueness of equilibrium relates to the elasticity of the type distribution.
\begin{assume}
\label{assume:elasticity}
The elasticity of the type distribution is weakly smaller than 2. Formally,
\[
\frac{f_S(z)z}{F_S(z)}\leq 2\,\forall\,z\in[0,1].
\]
\end{assume}
Using this assumption, we can prove the following:

\begin{prop}
\label{prop:symmetric_EQ}
Suppose $f$ is symmetric around $\ot$. When $p_R=\ot$ and $c<\bar{c}$, there is a symmetric interior equilibrium, $p_{Sl}^*(c)=1-p_{Sh}^*(c)$, where $$\frac{\partial p_{Sh}^*}{\partial c_S}>0>\frac{\partial p_{Sl}^*}{\partial c_S}.$$ Moreover, 
\[
\left.\frac{\partial p_{Sl}^*}{\partial p_R}\right|_{p_R=\ot}<0\,\,{ and }\,\,\left.\frac{\partial p_{Sh}^*}{\partial p_R}\right|_{p_R=\ot}<0.
\]
\end{prop}
\begin{proof}
Take the equilibrium conditions in a responsive equilibrium:

\[
\begin{array}{rcl}
C_L&=&-\left(p_{Sl}-\frac{\int_0^{{p_{Sl}}} z f(z) \,
   dz}{\int_0^{{p_{Sl}}} f(z) \, dz}\right)-c_S+\left|\frac{{\widehat{p}_R} \int_0^{{p_{Sh}}} z f(z) \, dz+(1-\widehat{p}_R) \int_{{p_{Sl}}}^1
   z f(z) \, dz}{{\widehat{p}_R} \int_0^{{p_{Sh}}} f(z) \, dz+(1-\widehat{p}_R)
   \int_{{p_{Sl}}}^1 f(z) \, dz}-p_{Sl}\right|,\\
C_H&=&-\left(\frac{\int_{{p_{Sh}}}^1 z f(z) \,
   dz}{\int_{{p_{Sh}}}^1 f(z) \, dz}-p_{Sh}\right)-c_S+\left|p_{Sh}-\frac{{\widehat{p}_R} \int_0^{{p_{Sh}}} z f(z) \, dz+(1-\widehat{p}_R) \int_{{p_{Sl}}}^1
   z f(z) \, dz}{{\widehat{p}_R} \int_0^{{p_{Sh}}} f(z) \, dz+(1-\widehat{p}_R)
   \int_{{p_{Sl}}}^1 f(z) \, dz}\right|.
\end{array}
\]
In a next step we simplify these, assuming (and later verifying) that a symmetric equilibrium exists. Letting $\widehat{p}_R=\ot$ and $p_{Sl}=\kappa=1-p_{Sh}$, and using the fact that
%
\begin{comment}
these become
\[
\begin{array}{rcl}
\left.C_L\right|_{p_R=\ot\wedge p_{Sl}=1-p_{Sh}=\kappa}&=&-\left(\kappa-\frac{\int_0^{\kappa} z f(z) \,
   dz}{\int_0^{\kappa} f(z) \, dz}\right)-c_S+\frac{\int_0^{{1-\kappa}} z f(z) \, dz+\int_{\kappa}^1
   z f(z) \, dz}{ \int_0^{{1-\kappa}} f(z) \, dz+
   \int_{\kappa}^1 f(z) \, dz}-\kappa\\
\left.C_H\right|_{p_R=\ot\wedge p_{Sl}=1-p_{Sh}=\kappa}&=&-\left(\frac{\int_{{1-\kappa}}^1 z f(z) \,
   dz}{\int_{{1-\kappa}}^1 f(z) \, dz}-(1-\kappa)\right)-c_S+(1-\kappa)-\frac{\int_0^{{1-\kappa}} z f(z) \, dz +\int_{\kappa}^1
   z f(z) \, dz}{\int_0^{{1-\kappa}} f(z) \, dz+
   \int_{\kappa}^1 f(z) \, dz}
\end{array}
\]
Now note that 
   
\end{comment}
%
\[
\frac{\int_0^{{1-\kappa}} z f(z) \, dz +\int_{\kappa}^1
   z f(z) \, dz}{\int_0^{{1-\kappa}} f(z) \, dz+
   \int_{\kappa}^1 f(z) \, dz}
   =\frac{\int_0^{1} z f(z) \, dz +\int_{\kappa}^{1-\kappa}
   z f(z) \, dz}{\int_0^1 f(z) \, dz+
   \int_{\kappa}^{1-\kappa} f(z) \, dz}
   =\frac{\ot +\int_{\kappa}^{1-\kappa}
   z f(z) \, dz}{1+
   \int_{\kappa}^{1-\kappa} f(z) \, dz}=\ot,
\]
where the last step follows from 
\[
\frac{\ot +\int_{\kappa}^{1-\kappa}
   z f(z) \, dz}{1+
   \int_{\kappa}^{1-\kappa} f(z) \, dz}=\ot\Leftrightarrow \ot +\int_{\kappa}^{1-\kappa}
   z f(z) \, dz=\ot+\ot \int_{\kappa}^{1-\kappa}
    f(z) \, dz\Leftrightarrow \frac{\int_{\kappa}^{1-\kappa}
   z f(z) \, dz}{\int_{\kappa}^{1-\kappa}
    f(z) \, dz}=\ot,
\]
which holds because of the symmetry around $\ot$ of $f$, we get
\[
\begin{array}{rcl}
\left.C_L\right|_{\widehat{p}_R=\ot\wedge p_{Sl}=1-p_{Sh}=\kappa}&=&
%-2\kappa+\frac{\int_0^{\kappa} z %f(z) \,
 %  dz}{\int_0^{\kappa} f(z) \, dz}-c_S+ \ot\\
\left| \frac{1}{2}-\kappa \right|
   -c_S+\frac{\int_0^{\kappa } z f(z) \, dz}{\int_0^{\kappa } f(z)
   \, dz}-\kappa,\\
\left.C_H\right|_{\widehat{p}_R=\ot\wedge 
p_{Sl}=1-p_{Sh}=\kappa}&=&\left| \frac{1}{2}-\kappa \right|
   -c_S-\frac{\int_{1-\kappa }^1 z f(z) \, dz}{\int_{1-\kappa }^1
   f(z) \, dz}+1-\kappa.
\end{array}
\]
Because $\ot>\kappa$, it follows that in the symmetric equilibrium we have
\begin{equation}
\label{eq:EQ_COND_L}
    \kappa= \frac{1}{4}-\frac{1}{2}c_S+\frac{1}{2}\frac{\int_0^{\kappa} z f(z) \,
   dz}{\int_0^{\kappa} f(z) \, dz}
\end{equation}
and
\begin{equation}
\label{eq:EQ_COND_H}
 \kappa=\frac{3}{4}-\frac{1}{2}c_S-\frac{1}{2} \frac{\int_{{1-\kappa}}^1 z f(z) \,
   dz}{\int_{{1-\kappa}}^1 f(z) \, dz}.
\end{equation}
We next show that \eqref{eq:EQ_COND_L} and \eqref{eq:EQ_COND_H} are equivalent and that there exists $\kappa\in(0,\ot)$ such that both are satisfied.
Equating \eqref{eq:EQ_COND_L} and \eqref{eq:EQ_COND_H}, we get
\[
\frac{1}{4}-\frac{1}{2}c_S+\frac{1}{2}\frac{\int_0^{\kappa} z f(z) \,
   dz}{\int_0^{\kappa} f(z) \, dz}=\frac{3}{4}-\frac{1}{2}c_S-\frac{1}{2} \frac{\int_{{1-\kappa}}^1 z f(z) \,
   dz}{\int_{{1-\kappa}}^1 f(z) \, dz}
\Leftrightarrow 
 \frac{\int_0^{\kappa} z f(z) \,
   dz}{\int_0^{\kappa} f(z) \, dz}+\frac{\int_{{1-\kappa}}^1 z f(z) \,
   dz}{\int_{{1-\kappa}}^1 f(z) \, dz}=1,
\]
which follows from the symmetry of $f$. Hence, it is sufficient to look at \eqref{eq:EQ_COND_L} to prove existence of a symmetric equilibrium. 

If $\kappa=0$, the  RHS of \eqref{eq:EQ_COND_L} is
\[
\frac{1}{4}-\frac{1}{2}c_S\geq 0.
\]
Hence, \eqref{eq:EQ_COND_L} is only satisfied when $\kappa=0$ if $c_S=\ot$.
If $\kappa=\ot$, the RHS of \eqref{eq:EQ_COND_L} is
\[
\frac{1}{4}-\frac{1}{2}c_S+\frac{1}{2}\frac{\int_0^{\ot} z f(z) \,
   dz}{\int_0^{\ot} f(z) \, dz}<\frac{1}{4}-\frac{1}{2}c_S+\frac{1}{2}\times \frac{1}{2}=\frac{1}{2}-\frac{1}{2}c_S\leq \frac{1}{2}.
\]
Because of continuity of \eqref{eq:EQ_COND_L},  there exists $\kappa\in[0,\ot)$ satisfying the equilibrium conditions simultaneously, implying a symmetric equilibrium exists for all $c_S\in[0,\ot]$.

Next we determine comparative statics. We need the following derivatives, which we evaluate at $\widehat{p}_R=\ot$ and $p_{Sl}=\kappa=1-p_{Sh}$:

\[
\begin{array}{rcl}
\frac{\partial C_L}{\partial p_{Sl}}&=&f(\kappa ) \left(\frac{\kappa }{\int_0^{\kappa } f(z) \, dz}-\frac{\int_0^{\kappa }
   z f(z) \, dz}{\left(\int_0^{\kappa } f(z) \, dz\right){}^2}+\frac{-\kappa 
   \left(\int_0^{1-\kappa } f(z) \, dz+\int_{\kappa }^1 f(z) \,
   dz\right)+\int_0^{1-\kappa } z f(z) \, dz+\int_{\kappa }^1 z f(z) \,
   dz}{\left(\int_0^{1-\kappa } f(z) \, dz+\int_{\kappa }^1 f(z) \,
   dz\right){}^2}\right)-2\\
\frac{\partial C_L}{\partial p_{Sh}}&=&-\frac{f(1-\kappa ) \left((\kappa -1) \left[\int_0^{1-\kappa } f(z) \, dz+ 
   \int_{\kappa }^1 f(z) \, dz\right]+\int_0^{1-\kappa } z f(z) \, dz+\int_{\kappa }^1 z
   f(z) \, dz\right)}{\left(\int_0^{1-\kappa } f(z) \, dz+\int_{\kappa }^1 f(z) \,
   dz\right){}^2}\\
\frac{\partial C_L}{\partial \widehat{p}_R}&=&-\frac{4 \left(\int_{\kappa }^1 f(z) \, dz\right) \int_0^{1-\kappa } z f(z) \, dz-4
   \left(\int_0^{1-\kappa } f(z) \, dz\right) \int_{\kappa }^1 z f(z) \,
   dz}{\left(\int_0^{1-\kappa } f(z) \, dz+\int_{\kappa }^1 f(z) \, dz\right){}^2}\\
\frac{\partial C_L}{\partial c_S}&=&-1
\end{array}
\]
and
\[
\begin{array}{rcl}
\frac{\partial C_H}{\partial p_{Sl}}&=&\frac{f(\kappa ) \left(\kappa  \left(\int_0^{1-\kappa } f(z) \, dz+\int_{\kappa }^1
   f(z) \, dz\right)-\int_0^{1-\kappa } z f(z) \, dz-\int_{\kappa }^1 z f(z) \,
   dz\right)}{\left(\int_0^{1-\kappa } f(z) \, dz+\int_{\kappa }^1 f(z) \,
   dz\right){}^2}\\
\frac{\partial C_H}{\partial p_{Sh}}&=&f(1-\kappa ) \left(\frac{1-\kappa }{\int_{1-\kappa }^1 f(z) \,
   dz}-\frac{\int_{1-\kappa }^1 z f(z) \, dz}{\left(\int_{1-\kappa }^1 f(z) \,
   dz\right){}^2}+\frac{(\kappa -1) \int_0^{1-\kappa } f(z) \, dz+(\kappa -1)
   \int_{\kappa }^1 f(z) \, dz+\int_0^{1-\kappa } z f(z) \, dz+\int_{\kappa }^1 z
   f(z) \, dz}{\left(\int_0^{1-\kappa } f(z) \, dz+\int_{\kappa }^1 f(z) \,
   dz\right){}^2}\right)+2\\
\frac{\partial C_H}{\partial \widehat{p}_R}&=&-\frac{4 \left(\left(\int_0^{1-\kappa } f(z) \, dz\right) \int_{\kappa }^1 z f(z) \,
   dz-\left(\int_{\kappa }^1 f(z) \, dz\right) \int_0^{1-\kappa } z f(z) \,
   dz\right)}{\left(\int_0^{1-\kappa } f(z) \, dz+\int_{\kappa }^1 f(z) \,
   dz\right){}^2}\\
\frac{\partial C_H}{\partial c_S}&=&-1.
\end{array}
\]
Define 
\[
  M=
  \left(
  \begin{array}{cc}
  \frac{\partial C_L}{\partial p_{Sl}}&\frac{\partial C_L}{\partial p_{Sh}}\\
  \frac{\partial C_H}{\partial p_{Sl}}&\frac{\partial C_H}{\partial p_{Sh}}
  \end{array}\right)   
\]
as well as
\[
\begin{array}{cc}
 M_L^{\widehat{p}_R}=
  \left(
  \begin{array}{cc}
  -\frac{\partial C_L}{\partial \widehat{p}_R}&\frac{\partial C_L}{\partial p_{Sh}}\\
  -\frac{\partial C_H}{\partial \widehat{p}_R}&\frac{\partial C_H}{\partial p_{Sh}}
  \end{array}\right)  &
  M_H^{\widehat{p}_R}=
  \left(
  \begin{array}{cc}
  \frac{\partial C_L}{\partial p_{Sl}}&-\frac{\partial C_L}{\partial \widehat{p}_R}\\
  \frac{\partial C_H}{\partial p_{Sl}}&-\frac{\partial C_H}{\partial \widehat{p}_R}
  \end{array}\right)  \\
  &\\
 M_L^c=
  \left(
  \begin{array}{cc}
  -\frac{\partial C_L}{\partial c_S}&\frac{\partial C_L}{\partial p_{Sh}}\\
  -\frac{\partial C_H}{\partial c_S}&\frac{\partial C_H}{\partial p_{Sh}}
  \end{array}\right)  &
  M_H^c=
  \left(
  \begin{array}{cc}
  \frac{\partial C_L}{\partial p_{Sl}}&-\frac{\partial C_L}{\partial c_S}\\
  \frac{\partial C_H}{\partial p_{Sl}}&-\frac{\partial C_H}{\partial c_S}
  \end{array}\right)  
\end{array}
\]
Then $\frac{\partial p_{Sl}}{\partial \widehat{p}_R}=\frac{\left|M_L^{\widehat{p}_R}\right|}{\left|M\right|}$, $\frac{\partial p_{Sh}}{\partial \widehat{p}_R}=\frac{\left|M_H^{\widehat{p}_R}\right|}{\left|M\right|}$, $\frac{\partial p_{Sl}}{\partial c_S}=\frac{\left|M_L^c\right|}{\left|M\right|}$, and $\frac{\partial p_{Sh}}{\partial c_S}=\frac{\left|M_H^c\right|}{\left|M\right|}$.

In the following we simplify the respective derivatives above such that we are able to sign them. First consider $\frac{\partial C_L}{\partial p_{Sl}}$ and note that 
\[\int_0^{1-\kappa } f(z) \, dz+\int_{\kappa }^1 f(z) \,
   dz=\int_0^{1} f(z) \, dz+\int_{\kappa }^{1-\kappa } f(z) \,
   dz=1+\int_{\kappa }^{1-\kappa } f(z) \,
   dz
\]
and 
\[\int_0^{1-\kappa } z f(z) \, dz+\int_{\kappa }^1 z f(z) \,
   dz=\int_0^{1}z f(z) \, dz+\int_{\kappa }^{1-\kappa }z f(z) \,
   dz=\ot+\int_{\kappa }^{1-\kappa }z f(z) \,
   dz.
\]
Using these and the fact that $f(1-\kappa)=f(\kappa)$ allows us to simplify six of the above derivatives:
\[
\begin{array}{rcl}
\frac{\partial C_L}{\partial p_{Sl}}&=&f(\kappa ) \left(\frac{\kappa }{\int_0^{\kappa } f(z) \, dz}-\frac{\int_0^{\kappa }
   z f(z) \, dz}{\left(\int_0^{\kappa } f(z) \, dz\right){}^2}+\frac{\left(\ot+\int_{\kappa }^{1-\kappa } z f(z) \,
   dz\right)-\kappa 
   \left(1+\int_{\kappa }^{1-\kappa } f(z) \,
   dz\right)}{\left(1+\int_{\kappa }^{1-\kappa } f(z) \,
   dz\right)^2}\right)-2\\
\frac{\partial C_L}{\partial p_{Sh}}&=&-f(\kappa )\frac{(\kappa -1) \left(1+\int_\kappa^{1-\kappa } f(z) \, dz\right)+\left(\ot+\int_\kappa^{1-\kappa } z f(z) \, dz\right)}{\left(1+\int_\kappa^{1-\kappa } f(z) \, dz\right)^2}\\
\frac{\partial C_L}{\partial \widehat{p}_R}&=&4\frac{
   \left(\int_{\kappa
   }^1 f(z) \, dz\right)\left(
   \int_0^{1-\kappa } z f(z)
   \,
   dz\right)-\left(\int_0^{1-\kappa }
   f(z) \, dz\right)\left(
   \int_{\kappa }^1 z f(z) \,
   dz\right)}{\left(1+\int_{\kappa }^{1-\kappa } f(z) \,
   dz\right){}^2}\\
\frac{\partial C_H}{\partial p_{Sl}}&=&f(\kappa )\frac{\kappa  \left(1+\int_\kappa^{1-\kappa } f(z) \, dz\right)-\left(\ot+\int_\kappa^{1-\kappa } z f(z) \, dz\right)}{\left(1+\int_\kappa^{1-\kappa } f(z) \, dz\right)^2}\\
\frac{\partial C_H}{\partial p_{Sh}}&=&f(\kappa ) \left(\frac{1-\kappa }{\int_{1-\kappa }^1 f(z) \,
   dz}-\frac{\int_{1-\kappa }^1 z f(z) \, dz}{\left(\int_{1-\kappa }^1 f(z) \,
   dz\right){}^2}+\frac{(\kappa -1) \left(1+\int_\kappa^{1-\kappa } f(z) \, dz\right)+\left(\ot+\int_\kappa^{1-\kappa } z f(z) \, dz\right)}{\left(1+\int_\kappa^{1-\kappa } f(z) \, dz\right)^2}\right)+2\\
\frac{\partial C_H}{\partial \widehat{p}_R}&=&4\frac{\left(\int_0^{1-\kappa
   } f(z) \, dz\right)\left(
   \int_{\kappa }^1 z f(z) \,
   dz\right)-\left(\int_{\kappa }^1
   f(z) \, dz\right)\left(
   \int_0^{1-\kappa } z f(z)
   \, dz\right)}{\left(1+\int_{\kappa
   }^{1-\kappa } f(z) \,
   dz\right){}^2}.
\end{array}
\]
Using
\eqref{eq:EQ_COND_L} and \eqref{eq:EQ_COND_H} as well as the facts that $\int_{0}^{\kappa } f(z) \,
   dz=F(\kappa)$ and $\int_{\kappa }^{1-\kappa } f(z) \,
   dz=1-2F(\kappa)$, the derivatives with respect to $p_{Sl}$ and $p_{Sh}$ can be expressed as follows:
\[
\begin{array}{rcl}
\frac{\partial C_L}{\partial p_{Sl}}&=&-f(\kappa ) \left(\frac{c_S+\kappa -\frac{1}{2}}{F(\kappa)}+\frac{ \kappa -\ot}{2 \left(1-
F(\kappa)\right)}\right)-2\\
\frac{\partial C_L}{\partial p_{Sh}}&=&-f(\kappa )\frac{\kappa-\ot}{2 \left(1-
F(\kappa)\right)}\\
\frac{\partial C_H}{\partial p_{Sl}}&=&f(\kappa )\frac{ \kappa -\ot}{2\left(1-F(\kappa)\right)}\\
\frac{\partial C_H}{\partial p_{Sh}}&=&f(\kappa ) \left(\frac{c_S+\kappa -\frac{1}{2}}{F(\kappa)}+\frac{ \kappa -\ot}{2 \left(1-
F(\kappa)\right)}\right)+2
\end{array}
\]
It is now easy to see that $\frac{\partial C_L}{\partial p_{Sl}}=-\frac{\partial C_H}{\partial p_{Sh}}$, $\frac{\partial C_L}{\partial p_{Sh}}=-\frac{\partial C_H}{\partial p_{Sl}}$, $\frac{\partial C_L}{\partial \widehat{p}_R}=-\frac{\partial C_H}{\partial \widehat{p}_R}$, and $\frac{\partial C_L}{\partial c_S}=\frac{\partial C_H}{\partial c_S}$. Using this in the determinants needed for comparative statics and simplifying yields
\begin{equation}
\label{eq:dpldp1}    
\frac{\partial p_{Sl}}{\partial \widehat{p}_R}=\frac{\partial p_{Sh}}{\partial \widehat{p}_R}=-\frac{\frac{\partial C_L}{\partial \widehat{p}_R}}{\frac{\partial C_L}{\partial p_{Sl}}+\frac{\partial C_L}{\partial p_{Sh}}}
\end{equation}
as well as
\begin{equation}
\label{eq:dpldcS} 
\frac{\partial p_{Sl}}{\partial c_S}=-\frac{\partial p_{Sh}}{\partial c_S}=\frac{1}{\frac{\partial C_L}{\partial p_{Sl}}-\frac{\partial C_L}{\partial p_{Sh}}}.
\end{equation}

We start with the former.
Because
\[
\begin{array}{rcl}
\dfrac{\partial C_L}{\partial \widehat{p}_R}<0&\Leftrightarrow&4\dfrac{
   \left(\int_{\kappa
   }^1 f(z) \, dz\right)\left(
   \int_0^{1-\kappa } z f(z)
   \,
   dz\right)-\left(\int_0^{1-\kappa }
   f(z) \, dz\right)\left(
   \int_{\kappa }^1 z f(z) \,
   dz\right)}{\left(1+\int_{\kappa }^{1-\kappa } f(z) \,
   dz\right)^2}<0\\
%&\Leftrightarrow&
%   \left(\int_{\kappa
%   }^1 f(z) \, dz\right)\left(
%   \int_0^{1-\kappa } z f(z)
%   \,
%   dz\right)<\left(\int_0^{1-\kappa }
%   f(z) \, dz\right)\left(
%   \int_{\kappa }^1 z f(z) \,
%   dz\right)\\
&\Leftrightarrow&
  \dfrac{\left(
   \int_0^{1-\kappa } z f(z)
   \,
   dz\right)}{\left(\int_0^{1-\kappa }
   f(z) \, dz\right)} <
   \dfrac{\left(
   \int_{\kappa }^1 z f(z) \,
   dz\right)}{\left(\int_{\kappa
   }^1 f(z) \, dz\right)}
\end{array}
\]
it  holds that $
\text{Sign}\left[\frac{\partial p_{Sl}}{\partial \widehat{p}_R}\right]=\text{Sign}\left[\frac{\partial C_L}{\partial p_{Sl}}+\frac{\partial C_L}{\partial p_{Sh}}\right]$. 
Hence,  we need to show that 
\begin{equation}
\begin{array}{c}
    \dfrac{\partial C_L}{\partial p_{Sl}}+\dfrac{\partial C_L}{\partial p_{Sh}}=\dfrac{f(\kappa ) (1-2 c_S-2 \kappa +2 c_S F(\kappa ))}{2 (1-F(\kappa )) F(\kappa )}-2<0\\
\Leftrightarrow \dfrac{f(\kappa ) (1-2 c_S-2 \kappa +2 c_S F(\kappa ))}{(1-F(\kappa )) F(\kappa )}<4.
\end{array}
\label{eq:dkdp1}
\end{equation}
To be able to determine if this is satisfied, we need to be able to say something about the possible values of $\kappa$ and $F(\kappa)$. For this we next prove an important lemma. Denote by $F_U(z)$ the CDF of the uniform distribution on $[0,1]$. Then: 

\begin{lem} (i)
\label{lemma:bounds}If $f(z)$ weakly increases on  $[0,\ot]$, then $F(z)\leq z$ for all $z\in[0,\ot]$. If $f(z)$ weakly decreases on  $[0,\ot]$, then $F(z)\geq z$ for all $z\in[0,\ot]$. If $F(z)\neq F_U(z)=z$, then the inequalities are strict.
 (ii) 
If $z\geq F(z)$ for all $z\in[0,\ot]$, 
then $\kappa\in\left[
\frac{1}{3}-\frac{2}{3}c_S,\ot-c_S\right]$. (iii) If $z\leq F(z)$ for all $z\in[0,\ot]$,  then $\kappa\in\left[0,\frac{1}{3}-\frac{2}{3}c_S\right]$.
\end{lem}
\begin{proof}
\noindent\textit{Part (i):}
Note that $F(0)=0$ and $F(\ot)=\ot$. Moreover, $F_{U}(z)=z$. If $f(z)$ is weakly increasing on $[0,\ot]$, $F''(z)=f'(z)\geq 0$ for $z\in[0,\ot]$. Hence, $F(z)\leq F_{U}(z)=z$ for $z\in[0,\ot]$. If $f(z)$ is weakly decreasing on $[0,\ot]$, $F''(z)=f'(z)\leq 0$ for $z\in[0,\ot]$. Hence, $F(z)\geq F_{U}(z)=z$ for $z\in[0,\ot]$.

\noindent\textit{Part (ii):}
Recall  condition \eqref{eq:EQ_COND_L}, pinning down $\kappa$ in the symmetric equilibrium.
If $F(z)=F_U(z)$, then $f(z)=1$, and thus $\frac{\int_0^{\kappa} z f(z) \,
   dz}{\int_0^{\kappa} f(z) \, dz}=\frac{\kappa}{2}$.  
Using this in \eqref{eq:EQ_COND_L}, $\kappa=\frac{1}{4}-\frac{1}{2}c_S+\frac{\kappa}{4}\Leftrightarrow \kappa=\frac{1}{3}-\frac{2}{3}c_S$. 
When $f(z)$ is weakly increasing on $[0,\ot]$ and $F(z)\neq F_U(z)$, then, compared to $F_U$, there is relatively more weight on higher values of $z$ than on lower values, and therefore we must have $\frac{\int_0^{\kappa} z f(z) \,
   dz}{\int_0^{\kappa} f(z) \, dz}\geq \frac{\kappa}{2}$. Hence, in this case,
\[
\kappa\geq\frac{1}{4}-\frac{1}{2}c_S+\frac{\kappa}{4}\Leftrightarrow \kappa\geq\frac{1}{3}-\frac{2}{3}c_S.
\]
Further, because $\frac{\int_0^{\kappa} z f(z) \,
   dz}{\int_0^{\kappa} f(z) \, dz}\leq \kappa$, 
\[
\kappa\leq\frac{1}{4}-\frac{1}{2}c_S+\frac{1}{2}\kappa\Leftrightarrow \kappa\leq\frac{1}{2}-c_S.
\]
Thus, if $f(z)$ weakly increases on $[0,\ot]$, $\kappa\in\left[\frac{1}{3}-\frac{2}{3}c_S,\frac{1}{2}-c_S\right]$.

\textit{Part (iii):}
Using similar steps we can show that if $f(z)$ is weakly decreasing on $[0,\ot]$, we must have $\kappa\leq\frac{1}{3}-\frac{2}{3}c_S$. The lower bound must be zero, and therefore, if $f(z)$ weakly decreases on $[0,\ot]$, then $\kappa\in\left[0,\frac{1}{3}-\frac{2}{3}c_S\right]$.
\end{proof}

The LHS of \eqref{eq:dkdp1} is strictly positive because $\kappa\leq\frac{1}{2}-c_S$ and it  increases in $f(\kappa)$. %Moreover, it follows from Assumption \ref{assume:elasticity} that $f(\kappa)\leq 2F(\kappa)/\kappa$. 
By Assumption \ref{assume:elasticity}, $f(z)\leq 2 F(z)/z$. Thus, if \eqref{eq:dkdp1} is satisfied when $f(\kappa)=2  F(\kappa)/\kappa$, then it generally holds. Substituting for $f(\kappa)$, we get the following:
\[
\begin{array}{c}
\dfrac{2F(\kappa)\left(1-2c_S-2\kappa+2c_S F(\kappa)\right)}{\kappa(1-F(\kappa))F(\kappa)}<4\Leftrightarrow 2\kappa (1-F(\kappa))>1-2c_S-2\kappa+2c_S F(\kappa)
\end{array}
\]
This is least likely to hold when $F(\kappa)$ is large. Hence let $F(\kappa)=\kappa$ (recall Lemma \ref{lemma:bounds}). Then,
\[
2\kappa-2\kappa^2>1-2c_S-2\kappa+2c_S\kappa\Leftrightarrow 4\kappa-2c_S\kappa-2\kappa^2>1-2c_S.
\]
The LHS of the inequality on the right increases in $\kappa$ because $4-2c_S-4\kappa>0\Leftrightarrow \kappa <1-\frac{1}{2}$. Hence, we can use the lower bound from Lemma \ref{lemma:bounds}:
\[
\begin{array}{c}
4\left(\frac{1}{3}-\frac{2}{3}c_S\right)-2c_S\left(\frac{1}{3}-\frac{2}{3}c_S\right)-4\left(\frac{1}{3}-\frac{2}{3}c_S\right)^2>1-2c_S\Leftrightarrow \frac{2}{9} (1-2 c_S) (5-c_S)>1-2c_S\\
\Leftrightarrow
\frac{2}{9} (5-c_S)> 1.
\end{array}
\]
This holds for all $c_S\in[0,\ot)$, hence proving this part of the  proposition.
 
Next consider \eqref{eq:dpldcS}. For this  to be negative, it must be true that 
\begin{equation}
\frac{\partial C_L}{\partial p_{Sl}}-\frac{\partial C_L}{\partial p_{Sh}}<0\Leftrightarrow \frac{(1-2 c_S-2 \kappa) f(\kappa )}{F(\kappa)}<4
\label{eq:dkdc}
\end{equation}
Using again Assumption \ref{assume:elasticity}, this must be true if
\[
\frac{(1-2 c_S-2 \kappa) 2F(\kappa)}{F(\kappa)\kappa}<4\Leftrightarrow
\frac{(1-2 c_S-2 \kappa) }{\kappa}<2\Leftrightarrow\kappa>\frac{1}{4}-\frac{1}{2} c_S.
\]
It follows from  Lemma \ref{lemma:bounds} that $\kappa\geq \frac{1}{3}-\frac{2}{3}c_S>\frac{1}{4}-\frac{1}{2}c_S$ for all $c_S\in[0,\ot)$, implying
this is  true. This proves the proposition.\end{proof}

\subsection{Example Accompanying Corollary 1: Maximal Polarization}
Corollary 1 states that our results from a unique and known receiver type remain valid also with multiple, heterogeneous receivers, if receivers are sufficiently homogeneous. 
In this section we show by way of a simple  but extreme example that homogeneity of the audience is not necessary for this result. In particular, we construct an example in which the audience is \textit{maximally polarized}, or heterogeneous, whereas the sender's types are uniformly distributed on $[0,1]$. We model  a maximally polarized audience by assuming that  $\widehat{p}_R\in\{0,1\}$. As we will see, $p_{Sh}^*>\widehat{p}_S^*(\emptyset)>p_{Sl}^*$, which holds true in any equilibrium with a  unique receiver type (see Lemma 1), is now always violated for one of the receiver types. Nevertheless,  the comparative static result from Corollary 1 still holds.

Formally, assume that the senders' worldview $F_S$ follows a continuous uniform distribution on $[0,1]$ and that receivers differ in their worldview $p_R$ such that there are $\mu$ receivers with $\widehat{p}_R=0$ and $1-\mu$ receivers with $\widehat{p}_R=1$.\footnote{Hence, to model maximum polarization, we implicitly assume that the parameters of the game are $\eta=1$ and $q=0$, as this produces $\widehat{p}_R\in\{0,1\}$ when $p_R\in\{0,1\}$.}  
%Receivers are thus maximally polarized on $[0,1]$. 
In this case, we can derive the equilibrium thresholds and beliefs in closed form. 

Receiver beliefs about the sender's worldview are
\[
\widehat{p}_S(0)=\frac{p_{Sl}}{2},\quad \widehat{p}_S(1)=\frac{1+p_{Sh}}{2},
\]
and
\[
\widehat{p}_S(\emptyset)=\frac{\widehat{p}_R \left(p_{Sh}^2+p_{Sl}^2-1\right)+1-p_{Sl}^2}{2 \widehat{p}_R
   (p_{Sh}+p_{Sl}-1)-2(1-p_{Sl})}.
\]

Equilibrium thresholds depend on $\mu$. If $\mu>\frac{1}{2}$,  $p_{Sh}^*>\widehat{p}_S^*(\emptyset)>p_{Sl}^*$ is satisfied for $\widehat{p}_R=0$, but for $\widehat{p}_R=1$, in equilibrium $p_{Sh}^*>p_{Sl}^*>\widehat{p}_S^*(\emptyset)$. The equilibrium thresholds in interior equilibrium are  equal to
\begin{equation}
    p_{Sl}^*=\frac{2 \mu  (\mu +1)-1-6 c_S}{2 \mu  (\mu +3)-2},\quad p_{Sh}^*=\frac{2c_S (2 \mu -1)+4 \mu ^2+2 \mu -1}{2 \mu  (\mu +3)-2}.
\end{equation}
This interior equilibrium exists iff $1/2 < \mu < 1$ and $0 \leq c_S < \frac{2 \mu-1}{10 + 4 \mu}$.
%$c_S<\frac{1}{14}$ and $\mu>\frac{1 + 10 c_S}{2 (1 - 2 c_S)}$. 

If $\mu<\frac{1}{2}$, $p_{Sh}^*>\widehat{p}_S^*(\emptyset)>p_{Sl}^*$ is satisfied for $\widehat{p}_R=1$, but for $\widehat{p}_R=0$, in  equilibrium we must have $\widehat{p}_S^*(\emptyset)>p_{Sh}^*>p_{Sl}^*$. The equilibrium thresholds in an interior equilibrium are equal to
\begin{equation}
    p_{Sl}^*=\frac{1-2 \left(c_S(1-2\mu) +\mu ^2\right)}{2 (\mu -5) \mu +6},\quad p_{Sh}^*=\frac{6 c_S-4 \mu +3}{2 (\mu -5) \mu +6}.
\end{equation}
Moreover, this interior equilibrium exists iff 
$0 < \mu < 1/2$ and $0 \leq c_S < \frac{2 \mu-1}{4 \mu-14}$.
%$c_S<\frac{1}{14}$ and $\mu<\frac{1-14 c_S}{2(1-2c_S)}$.

The comparative statics are as expected. Increasing $\mu$ shifts more weight toward receivers with lower worldviews. Hence, in line with the results from Proposition~5, in an interior equilibrium both thresholds should increase in $\mu$, which they do for all $\mu$ for which the equilibrium exists. Moreover, $p_{Sl}^*$ decreases in $c_S$ in an interior equilibrium, whereas $p_{Sh}^*$ increases in it.

In Figure~\ref{fig:WVmultR}, we plot both equilibrium thresholds and $\widehat{p}_S^*(\emptyset)$ for $\widehat{p}_R=0$ and $\widehat{p}_R=1$. We can see that (a) the thresholds always increase in $\mu$, and (b) the ranking of thresholds and beliefs after observing no signal are as discussed above.

\begin{figure}
    \centering
    \includegraphics[width=0.8\linewidth]{fig_mult.pdf}
    \caption{$p^*_{Sl}$ (lower solid and black curve) and $p^*_{Sh}$  (upper solid and black curve), as well as $\widehat{p}_S^*(\emptyset)$ for both $\widehat{p}_R=0$ (upper red and dashed curve) and $\widehat{p}_R=1$ (lower red and dashed curve)  and the expectation of $\widehat{p}_S^*(\emptyset)$ (dash-dotted, gray curve) for $\mu\in[0,1]$ and $c_S=0$.}
    \label{fig:WVmultR}
\end{figure}

%As a first step, beliefs as functions of the equilibrium thresholds $p_{Sl}$ and $p_{Sh}$ equal.

%\[
%\begin{array}{rcl}
%\widehat{p}_S(0) &=& \dfrac{p_{Sl}}{2}, 
%\qquad
%\widehat{p}_S(1) = \dfrac{1+p_{Sh}}{2}, \\[1.1em]
%\widehat{p}_S(\emptyset) &=& 
%\dfrac{1 - p_{Sl}^2 + p_R (p_{Sh}^2 + p_{Sl}^2-1)}{2 - 2 p_{Sl} + 2 p_R (p_{Sh} + p_{Sl}-1)}.
%\end{array}
%\]
%Furthermore, $\widehat{p}_S(\emptyset)$ is always larger for a receiver with $p_R=0$ and for $p_R=1$.  In a Responsive Equilibrium, the following two indifference conditions must hold and determine $p_{Sl}$ and $p_{Sh}$:
%\begin{eqnarray}\label{wwIndif1}
%C_l &\equiv& \dfrac{p_{Sl}}{2} 
%+ \mu ( \widehat{p}_S(\emptyset|p_R=0) - p_{Sl} )+(1-\mu)\left| \widehat{p}_S(\emptyset|p_R=0) - p_{Sl} \right|  = 0, \\[0.6em]
%C_h &\equiv& -\left| p_{Sh} - \widehat{p}_S(1) \right| - c_S 
%+ \int_0^1 \left| \widehat{p}_S(\emptyset) - p_{Sh} \right| \, dF_R(p_R) = 0.
%\label{wwIndif2}
%\end{eqnarray}
%where we used $\widehat{p}_S(\emptyset|p_R=0) > p_{Sl}$ and $\widehat{p}_S(\emptyset|p_R=1) < p_{Sh}$ always hold

\end{document}
